# Supplementary material for: Gazealytics: A Unified and Flexible Visual Toolkit for Exploratory and Comparative Gaze Analysis
Source: arXiv:2303.17202 source file (2023-04-26)
Supplement: Supplementary file 1 [file appendix.tex]

\section{Gallery}
\label{sec:appendix}
\begin{figure}
    \centering
     \subfigure[Example of hypothesis driven exploration]{
    \includegraphics[width=1.0\textwidth]{figures/hypothesis_driven.pdf}
    }
    
    \Description[Example of hypothesis driven exploration]{Example of hypothesis driven exploration}
    \caption[]{Example of hypothesis driven exploration
    }
    \label{fig:supple_hypothesis_driven_example}
\end{figure}
\begin{figure}
    \centering
     \subfigure[Example of observational study recorded using a mobile eye tracker]{
    \includegraphics[width=1.0\textwidth]{figures/aemo.png}
    }
    
    \Description[Example of layout and matrix visualisation]{Example of observational study recorded using a mobile eye tracker}
    \caption[]{Example of observational study recorded using a mobile eye tracker
    }
    \label{fig:aemo}
\end{figure}

\begin{figure}
    \centering
     \subfigure[Comparison of average mean fixation and saccade length in the same session of two operators performing their daily tasks]{
    \includegraphics[width=1.0\textwidth]{figures/aemo_visual-metrics.pdf}
    }
    
    \Description[Example of layout and matrix visualisation]{Example of \webveta{} GUI layout showing data panel (upper left), spatial canvas, metric canvas, timeline canvas, and control panel (right)}
    \caption[]{Comparison showing differences in mean fixation and saccade length in the same session of two operators performing their daily tasks. 
    }
    \label{fig:aemo2}
\end{figure}
\begin{figure}
    \centering
     \subfigure[Example using video linked with TWIs]{
    \includegraphics[width=0.8\textwidth]{figures/P05_example.png}
    }
    
    \Description[Example of video linked with a selected TWI]{Example of \webveta{} GUI layout showing data panel (upper left), spatial panel, video panel, timeline panel, and control panel (right)}
    \caption[]{Example of \webveta{} GUI layout showing data panel (upper left), spatial panel, video panel, timeline panel, and control panel (right).
    }
    \label{fig:matrix_visualisation}
\end{figure}

\textit{Exploration of gaze patterns in an observational study}
We show examples recorded from a mobile eye tracker.
Data was from a previously published study, recorded in an Australian Energy Control Room~\cite{goodwin2022veta}. 
In this example, gaze semantic mapping to a stationary field of view was done beforehand. 
We annotated fixations and scanpaths with AOIs using \webveta{}. 

\section{Interactive visualisation design}
\label{sec:supple_interaction_design}
% In order to highlight how \webveta{} supports a highly flexible analysis. We also highlight previous work with their limitation. 
% We also relate to Kurzhals et al.’s eye tracking task taxonomy~\cite{kurzhals2017task}.
% \begin{figure}
%     \centering
%      \includegraphics[width=0.8\textwidth]{figures/haar_case_study.pdf}
    
%     \Description[]{}
%     \caption[]{Interactive manipulation of AOIs (using the space view) for labelling fixations, linked with sample-AOI relationships with a hit-any-AOI-rate (HAAR) metric. 
%     This metric is independent of AOIs. 
%     It improves the effect of AOI uncertainty by improving HAAR from 77\% (left) to 88\% (middle), and finally to 93\% (right) for a more robust AOI definition. The scarf plot at the bottom right shows that fixations at the gray area (bottom left) were mapped to clear AOis: aoi4 and aoi6. 
%     \label{fig:case_study_haar}
%     }
% \end{figure}

In the following, we describe \webveta{}'s interactive visualisations, grouped into Encode, Manipulate, and Introduce categories~\cite{brehmer2013multi}. 
These categories are also used in Table 1 of the main paper.

% Prior work also applies these categories to classify interaction data~\cite{Blascheck2016}.
% We refer the readers to supplementary materials for technical implementaion details of each functionality including multiple coordinated views, visual metrics, and interactive GUI design. 
\subsection{Encode} \webveta{} supports both AOI- and point-based visual encoding of gaze data mapped onto visualisations.

\subsection{Manipulate} \webveta{} supports a comprehensive set of tools for alterations of visual elements.

\textit{Select.} 
Focus-and-context interaction allows selecting an AOI and gaining an overview of surrounding spatial context of fixations before/after glancing an AOI~\cite{goodwin2022veta,netzel2016interactive}, as shown in~\autoref{fig:case_study_haar} (top), where density map of a selected sample P20 is shown. 
We further provide brushing  \& linking with complementary views. ~\autoref{fig:case_study_haar} (middle) shows that the linked hit-any-AOI-rate (HAAR) metric for an initial AOI definition yields a much lower value (77\%) than the rest of the samples. This could affect the quality of eye tracking data analysis~\cite{wang2022impact}. 
% Selection of a sample is directly over a mouse click on a particular matrix row/column or on a sample from the scarf plot. 
Further exploration and adjusting AOI definitions with the help of density map, visual metrics and scarf plot improves HAAR to 93\%, as seen in~\autoref{fig:case_study_haar} (middle, bottom). 
% Brushing over a scarf plot of a particular sample, bin of a histogram, or a matrix cell shows selected visual elements in complementary views. 
% Brushing over a bin of histogram shows where and when the saccades of group of them are in the spatial context and when it occurs. This helps to gain context of where and when the frequently short saccades occur which may result from cognitive load~\cite{netzel2014comparative}, likewise for long visual searches that may take greater mental effort~\cite{goodwin2022veta}.
This also applies to brushing over arbitrary matrix relationships, such as between a sample (group) and an AOI (group), which highlights group fixations (), saccades, or their transitions between AOIs (groups) (FigureX). Brushing over a multi-similarity matrix shows linear red and blue scale in the spatial view (FigureX) for pairwise differences.
Hovering over a scarf plot shows temporal sequence of scanpaths on the spatial view. 
 
% link-and-brush is also applied to bins of histogram, timeline of a particular sample (scarf plot) to highlight visuals in the complementary view.

% AOI timeline show AOIs as rows and we highlight selected AOI white and the rest will show gray, to make it salient to observe patterns [x]. 

% The matrix colour encodes a linear red/blue gradient. 

\textit{Navigate.}
Selected group view shown in~\autoref{fig:group_level_matrix_timeline.pdf}
focuses on a trial to compare across all the samples.
Existing work supports navigating between overview or detail-on-demand by selecting a specific timespan for video stimuli~\cite{kurzhals2014iseecube}. 
% navigation aggregates density map and shows scanpath details of each individual user~\cite{menges2020visualization}.
We extensively support a flexible navigation between overview and detailed views by six levels-of-detail by toggling two buttons (data dimensions: samples and TWIs) of three states (all, selected group, selected individual). The top row of \autoref{fig:webveta_overview}(b) indicates the current coordinated views are in detail mode where ``all-samples, all-TWIs'' are in place. 
A different view where sample data is aggregated into two groups, using ``selected-sample-group and selected-TWI-group'' is shown in~\autoref{fig:matrix_visualisation}.
% We achieve this by a matrix-based overview, with group-level visualisations. For example, 
% Figure XX shows overview, detailed view, group view.
One can navigate small-multiple views within the matrix where ``selected-TWI-group'' and the desired group are selected. This gives an overview in the matrix with grouped TWIs associated with a number of repeated measures of a particular experimental condition. Toggling the button to ``selected TWI'' switches to a detailed view when triggering a within-subject comparison over a selected trial. 
% Last but not least, by cropping a specific area from the spatial view, a user can change the viewport by zooming in, useful when gaze relationships only occur on a small regions of a given stimuli. Metrics are re-calculated with respect to the cropped region and visualisations are generated accordingly. A user can undo cropping to return previous viewport, or reset to the original uncropped viewport. 

% None of existing research or commercial tools supports visual cropping. 

% with a button simple rotating state by showing all samples, selected sample group (aggregating all samples , all TWIs view, or selected sample group, selected TWI group view. overview aggregated spatial, matrix/histogram view or detailed views via 

% Xx characterized insights into overview, pattern, group, or detail

\textit{Arrange.} 
Many existing visual tools do not always support changing ordering of data representation or layout of visualisations (\autoref{tab:toolscompare}). Some visualisations rarely change order~\cite{kurzhals2014iseecube}. Some have limited screen space allocated to a specific view~\cite{Blascheck2016}. The order of AOIs in these sequence plots is often tied to the order they appear in the dataset~\cite{Blascheck2016,kurzhals2014iseecube}. 
By contrast, order of data presentation (samples, AOIs, TWIs) in \webveta{}'s coordinated views is constantly synchronised to maintain a consistent view, with the order representation automatically rearranged via optimal matrix reordering, or sorting of data elements initiated by a user from data control or mouse click on a matrix row/column.
We further provide the flexibility in resizing the layout of each coordinated view to allow to allocate more or less space such as for matrix or timeline for specific analytical needs (\autoref{fig:webveta_overview}).
% by a responsive GUI, which maintains aspect ratios for all the coordinated views on changing window size. 
% To address screen space allocated for a view, we also provides the ability to 
% manually lay out each view to, e.g., accommodate more data elements in a matrix or timeline for specific analytical needs. 
% This flexibility addresses the limitation of available space for accommodating more data elements in an visualisation when multiple coordinated views is used [x].
% Order of data representation of samples, AOIs, and TWIs has an effect in all coordinated views to present a consistent view. 

% Global optimisation algorithms cluster these variables to reveal group patterns in the matrix. A user can also use local sorting, which sort all the rows, columns by a selected row or column in increasing or decreasing order according to the selection.

% ISeeCube and VA2 both "Ordering the AOIs by their first appearance results" 

% By contrast, we use matrix reordering to synchronise the order of AOIs based on the orders that reveal block patterns; further, a user can manually arrange the order or click on the row or column to sort the order according to the metric value contained in matrix cell. 

\textit{Change.} 
% \webveta{} supports multiple ways of configuring a TWI. An optional fourth column -- TWI name can be provided in aforementioned TSV file. A user can label a sequence of gaze points as a specific timespan (TWI) of an experimental condition. 
Unlike most existing research tools (\autoref{tab:toolscompare}), size of fixation, shape of density plots, colour scheme and its alpha values of visualisations is changable, at individual- or group-level. 
% flexible in custimising to match the colour definition of users' existing experimental conditions. 
In \webveta{}, a TWI can be manipulated dynamically by left mouse click to drag and drop a timespan over the timeline, with an effect on linked visual metric view and spatial view.
% The brightness for the background image can be controlled by a slider in the Overview tab.
% A fixation is represented by a circle. Its size is changeable from the control panel.
% The colour of the fixations, saccades visualisations encodes group colour.
% Density kernel maps can be altered by shapes (Bell curve, inverse square, pyramid, cone, flat) and a blur radius to control the degree of density kernel estimation. 
Animated spatiotemporal view filters data in a chronological order, allowing for animating the change in the gaze data over time. 
% A user can customise a \textbf{density map} for each sample or sample groups, using a kernel-density estimation based on the fixations within the selected time interval. Kernel shape and width can both be controlled. Colour depends on the group value of the sample. Detailed functions are in supplementary material pdf.

% We adopt qualitative colour scheme using ColorBrewer~\cite{harrower2003colorbrewer} as prior work does~\cite{kurzhals2014iseecube}, for each data dimension. Group of elements is also distinguishable with a colour class. 

% encode multivariate data, i.e., sample, AOI, TWI visually distinguishable, 
% We adopt qualitative color scheme from ColorBrewer~\cite{harrower2003colorbrewer} and use different class set for samples, AOIs, TWIs. Group of these variables use the same class set, but the order of colour is reversed.

% This has an effect on the fixation and saccade marks on the spatial view and the timeline, but not any of the metrics.

% Left mouse click and drag-and-drop over timeline triggers to create a new TWI if no TWI time interval is hit. Othewise, it shifts current TWI to a different start time based on the mouse moving distance. 

\textit{Filter.}
Supported by most tools, a user can turn on/off any visual overlay, or samples, AOIs, TWIs, with an effect on data re-processing, including metrics of data aggregation re-calculation and visualisations generation.

\textit{Aggregate.}
Most existing work do not visually aggregate metrics for multiple data dimensions. They exclusively aggregate one of AOIs~\cite{blascheck2016aoi}, samples [x], or TWIs [x]. Much work cluster samples but do not aggregate them in visual elements~\cite{Blascheck2016,kurzhals2014iseecube}. Furthermore, data granularity shown is unchanged as a result of data aggregation~\cite{brehmer2013multi}.
\webveta{} allows a user to aggregate fixations,  visitations [x], density distribution, saccade transition counts, etc, from two or multiple samples, spatial aggregation of metrics in AOIs, temporal aggregation of metrics in TWIs. 
% Visual metrics are automatically re-calculated as a result of data grouping.
% change the granularity of visualisation elements: AOIs, samples, TWIs
% Directional saccade bundling is supported and controlled by rigidity and heat parameters in the GUI~\cite{hurter2011moleview}. 
% Sliders are used frequently to change granularity of timespan where TWI data and metrics being computed is changed dynamically.
% Left mouse click and drag-and-drop over timeline triggers to create a new TWI if no TWI time interval is hit. Othewise, it shifts current TWI to a different start time based on the mouse moving distance. 

\subsection{Introduce} \webveta{} provides an easily configurable interface for integration into analysts' existing workflows.

\textit{Annotate.} 
% AOI labelling (parameter manipulation)
A gaze point is assigned to an AOI when it lies inside the bounding box of the AOI. Left-click on AOI for drag-and-drop selects on the boundary (in the case of rectangular AOI) or vertices (in the case of polygon AOI) and enables AOI resizing and shape manipulation.  
% Overlapping AOIs will label a fixation based on the highest precedence order from the AOI list that where the fixation hits. 
Text annotation over spatial view is also supported (FigureX).

% In general, the analysis of eye-tracking records from time dependent data can either be achieved by watching the video with the aforementioned visualization methods, or by statistical analysis of AOIs and gaze data. Watching the whole video to find interesting sequences can be time-consuming and exhausting for the analyst. Statistical analysis of AOIs requires either a reliable detection algorithm to find them, or tedious manual editing.

% It supports unlabelled gaze data, with the flexibility in dynamically annotating them with AOIs while visually inspecting the impact of manipulating AOIs on visual metrics (such as AOI uncertainty metrics) and on the context of previous and subsequent fixations visiting AOIs, to arrive at more robust AOI definitions. 
% Interactive data analysis will be described in relevant subsections.

\textit{Import.}
% Import samples is supported by all the methods so we skip this entry in~\autoref{tab:toolscompare}.
% Except importing samples, most existing visual analytics tools do not simultaneously support importing AOIs, TWIs and more importantly their grouping information (\autoref{tab:toolscompare}), limiting their flexibility in integrating with existing workflow. 
All of the data dimensions, including sample, AOIs, TWIs and their group IDs (GIDs) could be imported from either json or TSV files. 
TWIs could be imported via specifying in the fourth column of a gaze sample TSV file, or a separate tsv file of start and end timestamp. TWI grouping could be imported via a json setting file.

% \webveta{} supports multiple ways of configuring a TWI. An optional fourth column -- TWI name can be provided in aforementioned TSV file. A user can label a sequence of gaze points as a specific timespan (TWI) of an experimental condition. 
% TWI can also be created dynamically by left mouse click to drag and drop a timespan over the timeline.

\textit{Derive.}
% While automatic clustering algorithms are applied~\cite{Blascheck2017,kurzhals2015gaze}, they typically do not derive new attributes as a result of clustering, rather, dendrogram is commonly used to highlight hierarchical clustering of individual samples. 
% The order of data representation or alter granularity of data that derives new attributes~\cite{brehmer2013multi}. 
% To improve the flexibility in visual exploration, we adopt the approach of optimising visual arrangement of data to reveal patterns. 
New attributes such as group-level visual metrics could be derived from \webveta{} and remain persistent.

\textit{Record/Produce.}
\webveta{} supports exporting multiple data files in a single zip file for consumption in external tools, manipulated externally, and re-imported into \webveta{} for gaze replay. Exportable data includes, but is not limited to, all the visualisations, AOIs, TWIs, samples hitting or missing AOIs outcome, fixation, saccade, and scanpath metrics, data grouping, and all the parameter configurations.
